# Supplementary material for: Joint Deblurring and 3D Reconstruction for Macrophotography
Source: arXiv:2510.01640 source file (2025-10-02)
Supplement: Supplementary file 1 [file X_suppl.tex]

% \clearpage
% \setcounter{page}{1}
% \maketitlesupplementary

\section{Imaging Laws in Geometric Optics.}
\label{sec:optics}

This section provides supplementary information and analysis about the mentioned imaging laws~\cite{li2005applied, hecht2017optics} and Circle of Confusion(CoC) in macrophotography. 

As shown in Fig.~\ref{fig:optics}, assume that the focal length of the camera lens is \(f\), the distance between the camera film and the lens is \(F\), and the effective aperture of the lens is \(A\), there exists a plane in space at a distance \(d_0\) from the camera lens, so that all light rays emitted from a point on the plane will converge to a point on the film after passing through the lens. The distance \(d_0\) of the plane should satisfy
\begin{equation}
  \frac{1}{d_0} + \frac{1}{F} = \frac{1}{f}.
  \label{eqsup1}
\end{equation}

When the point \(\mathbf{p}\) leaves the plane, assuming that the distance between the point \(\mathbf{p}\) and the camera lens is \(d_\mathbf{p}\) at this time, the convergence point of the light rays emitted from the point behind the lens will not be on the film. This makes the projection of the point \(\mathbf{p}\) on the film a circular area with a radius of \(\sigma_\mathbf{p}\). Assuming that the distance between the convergence point of the light rays emitted from the point behind the lens and the lens is \(F_{\mathbf{p}}\), then according to the principle of similar triangles, \(\sigma_\mathbf{p}\) satisfies
\begin{equation}
  \frac{\sigma_\mathbf{p}}{A/2} = \frac{|F_{\mathbf{p}}-F|}{F_{\mathbf{p}}}.
  \label{eqsup2}
\end{equation}

Similar to \(d_0\), \(F_{\mathbf{p}}\) also satisfies
\begin{equation}
  \frac{1}{d_\mathbf{p}} + \frac{1}{F_\mathbf{p}} = \frac{1}{f}.
  \label{eqsup3}
\end{equation}

Combining Eq.~\eqref{eqsup1}, Eq.~\eqref{eqsup2}, and Eq.~\eqref{eqsup3}, then eliminating \(F\) and \(F_{\mathbf{p}}\), we can get the relationship between \(\sigma_{\mathbf{p}}\) and scene parameters:
\begin{equation}
  \sigma_\mathbf{p}=\frac{1}{2}fA\frac{|d_\mathbf{p}-d_0|}{d_\mathbf{p}(d_0-f)}= \frac{fA}{2d_{\mathbf{p}}(d_0-f)}\cdot\epsilon_{\mathbf{p}}.
  \label{eqsup4}
\end{equation}

Generally, \(\sigma_{\mathbf{p}}\) with the same \(\epsilon_{\mathbf{p}}\) in macro scenes is much larger than that in normal scenes. 

According to Eq.~\eqref{eqsup4}, the sensitivity of \(\sigma_{\mathbf{p}}\) to \(\epsilon_{\mathbf{p}}\) relies on the term \(\frac{fA}{2d_{\mathbf{p}}(d_0-f)}\). In normal scenes, a typical setting is that \(f=50\text{mm}, A=1/2.8\) and \(d_0\) is about several meters, while \(d_\mathbf{p}\) varies around \(d_0\) with several tens cm. However, in macro scenes, the typical setting is usually \(f=100\text{mm}, A=1/2.8\) and \(d_0\) is just several centimeters, while \(d_\mathbf{p}\) varies around \(d_0\) with several millimeters. These differences make that \(\sigma_{\mathbf{p}}\) with the same \(\epsilon_{\mathbf{p}}\) in macro scenes is hundreds of times larger than that in normal scenes. Therefore, defocus blur in macrophotography is usually unavoidable.

\section{Guided Filter-Based Focus Region Detection}
\label{sec:gfif}

\begin{figure}
    \centering
    \includegraphics[width=\linewidth]{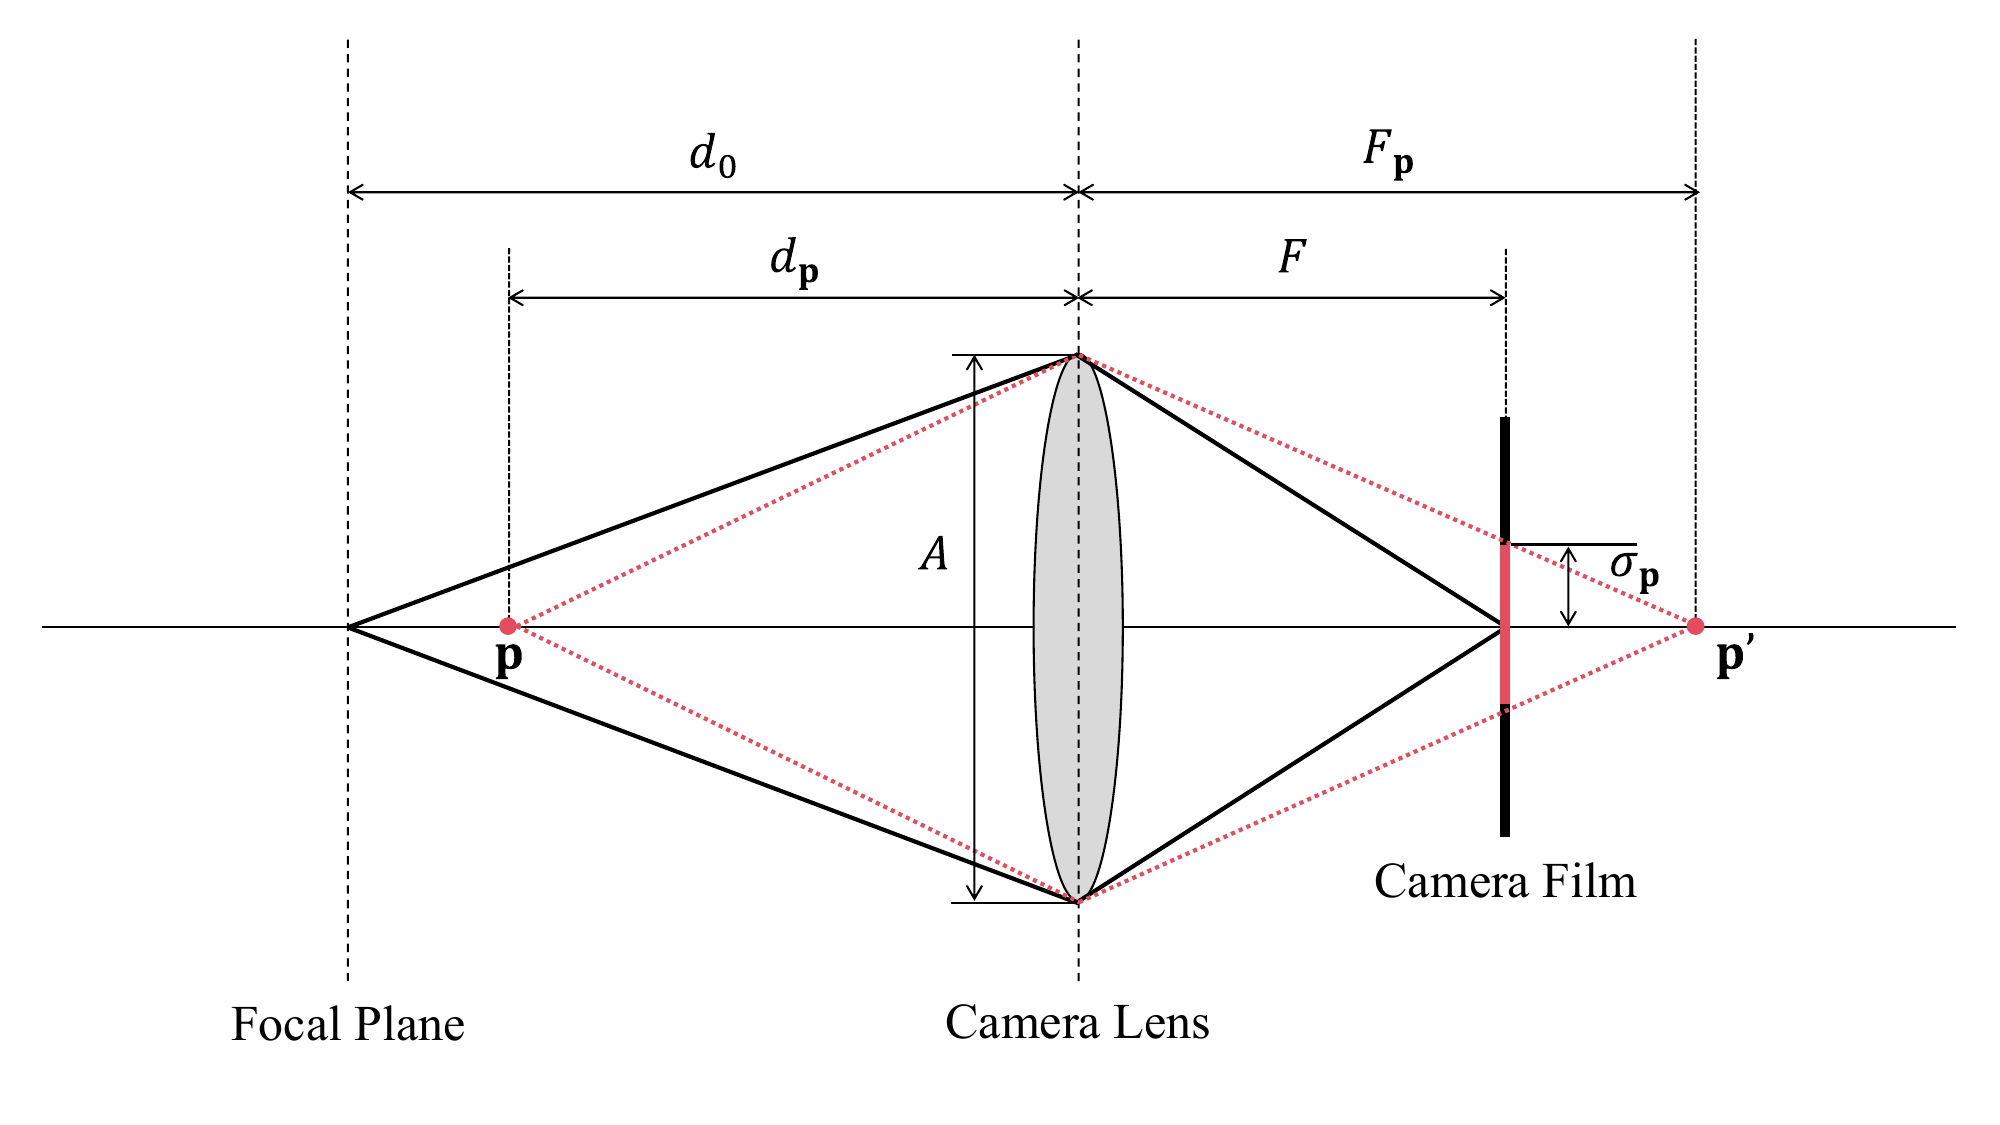}
    \vspace{-20pt}
    \caption{\textbf{The imaging model of an ideal thin lens.} Points far from the focal plane will be projected as circular areas on the film. In microscopic scenes, even a small distance away from the focal plane will make the radius of the circular area very large.}
    \label{fig:optics}
    \vspace{-0.2cm}
    % \vspace{-8pt}
\end{figure}

We introduce an algorithm~\cite{QIU2019} into our method to calculate a clarity mask \(\mathbf{M}\) for each input image. This section details the pipeline of this algorithm.

\begin{figure}[h]
% \vspace{-1em}
    \centering
    \includegraphics[width=\linewidth]{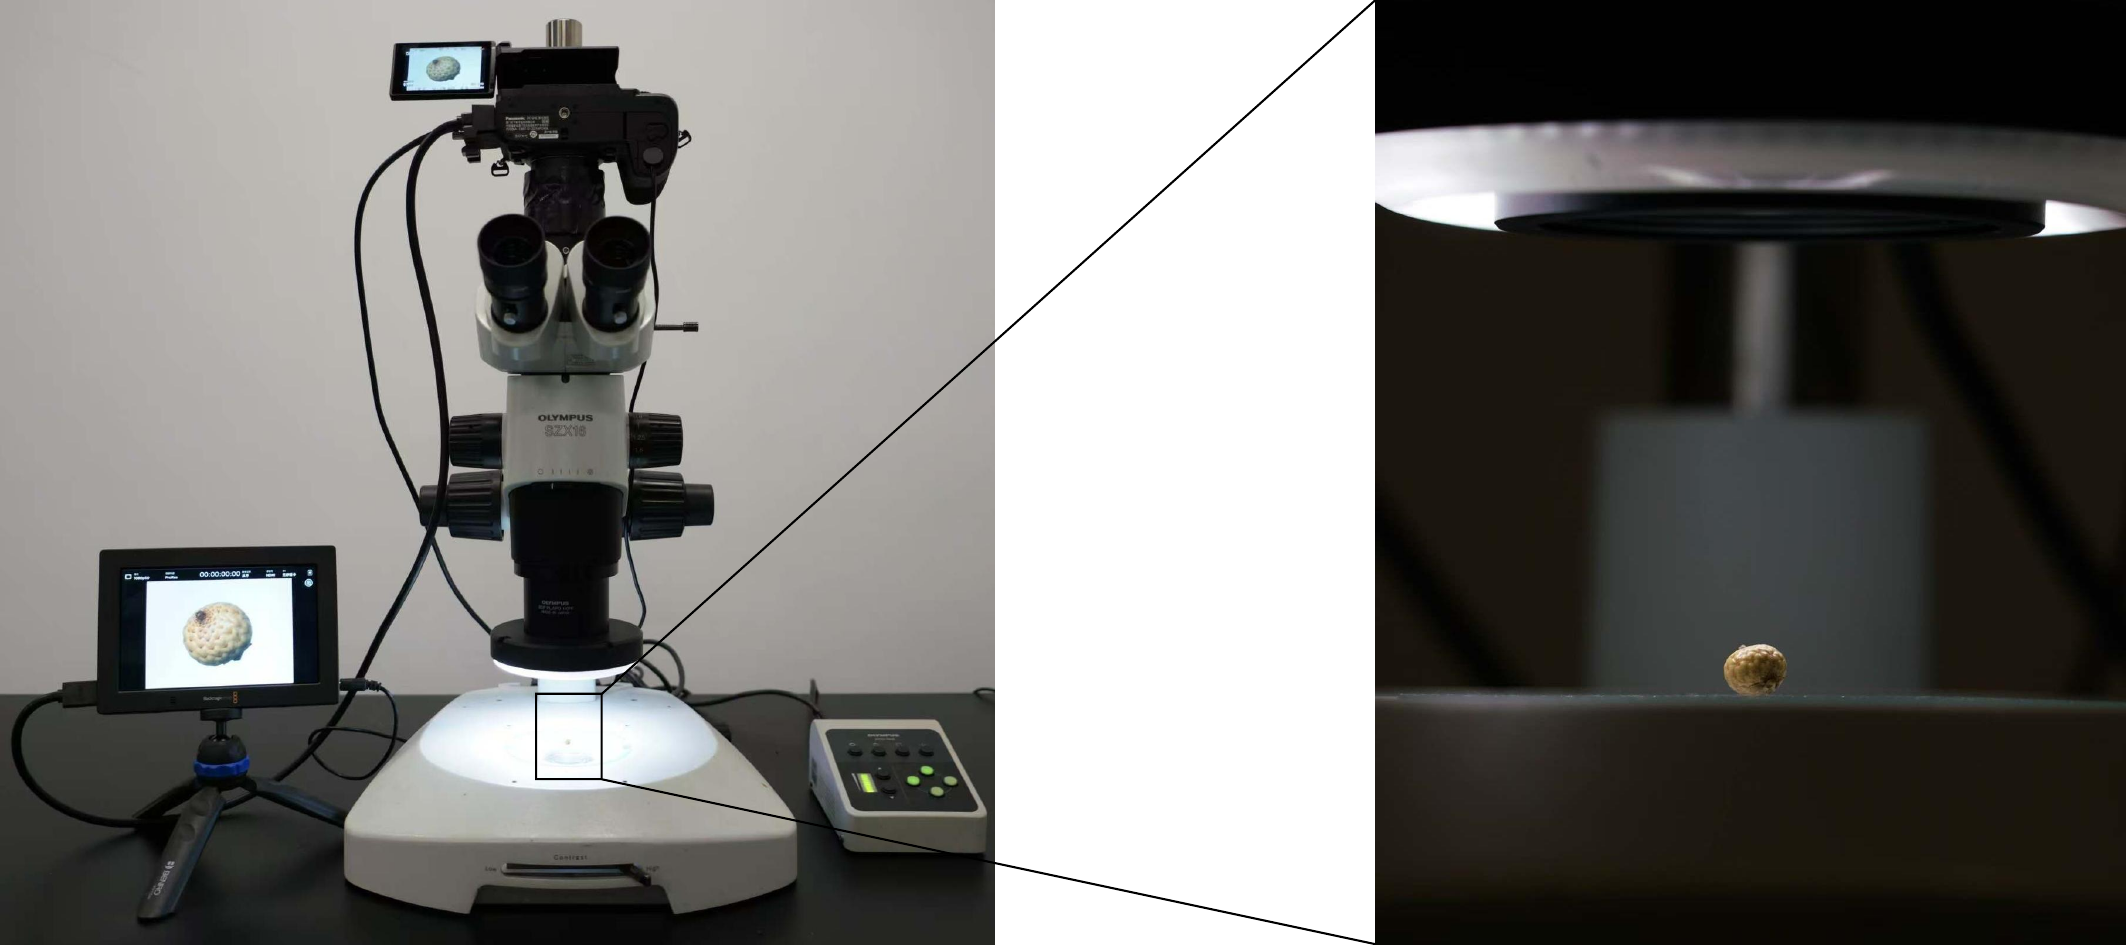}
    \vspace{-20pt}
    \caption{\textbf{Microscope with turnable device and captured object}}
    \label{fig:rebuttal_scene}
    % \vspace{-0.2cm}
    % \vspace{-1em}
    % \vspace{-2em}
\end{figure}

%& Ablation Study Visual Comparisons
\captionsetup[subfigure]{labelformat=empty}
\begin{figure*}[htb!]
    \setlength{\abovecaptionskip}{3pt}
    \setlength{\tabcolsep}{0.5pt}
    \centering
    \small
    \begin{tabular}[b]{cccccccc}
        % \hline
         Novel View & Defocus & w/o depth & w/o mask & w/o stages & w/o BlurNet & Ours & GT\\

        \begin{subfigure}[b]{0.2\linewidth}
            \includegraphics[width=\textwidth]{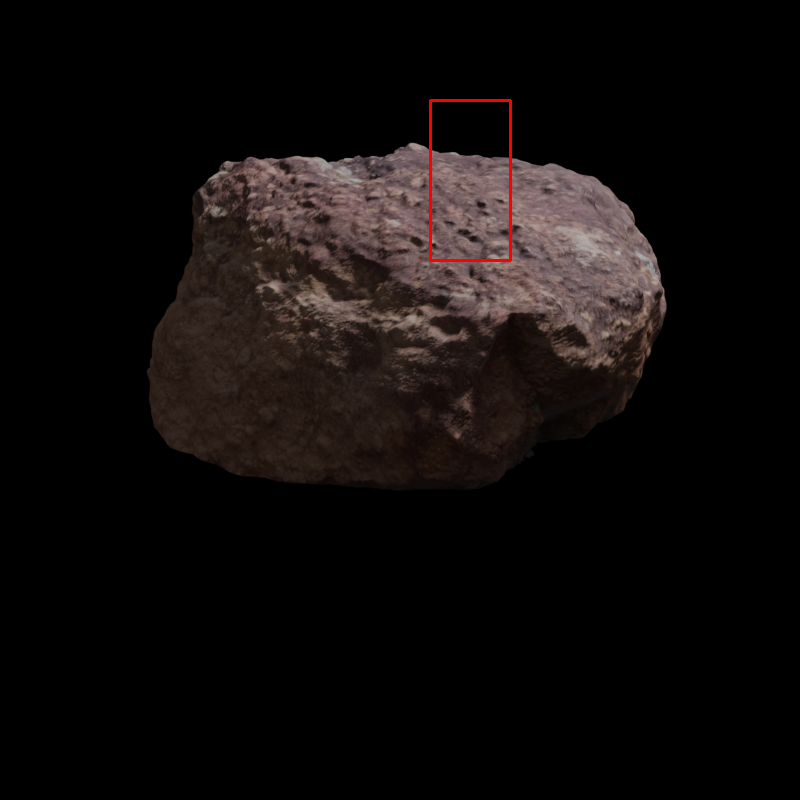}
            % \caption{Grain}
        \end{subfigure} &
        \begin{subfigure}[b]{0.1\linewidth}
            \includegraphics[width=\textwidth]{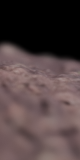}
            % \caption{}
        \end{subfigure} &  
        \begin{subfigure}[b]{0.1\linewidth}
            \includegraphics[width=\textwidth]{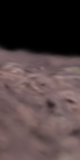}
            % \caption{}
        \end{subfigure} &
        \begin{subfigure}[b]{0.1\linewidth}
            \includegraphics[width=\textwidth]{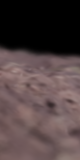}
            % \caption{}
        \end{subfigure} &
        \begin{subfigure}[b]{0.1\linewidth}
            \includegraphics[width=\textwidth]{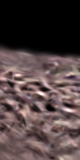}
            % \caption{}
        \end{subfigure} &
        \begin{subfigure}[b]{0.1\linewidth}
            \includegraphics[width=\textwidth]{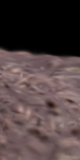}
            % \caption{}
        \end{subfigure} &   
        \begin{subfigure}[b]{0.1\linewidth}
            \includegraphics[width=\textwidth]{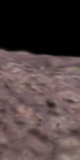}
            % \caption{}
        \end{subfigure} &  
        \begin{subfigure}[b]{0.1\linewidth}
            \includegraphics[width=\textwidth]{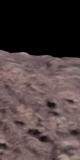}
            % \caption{}
        \end{subfigure} \\ 

        PSNR/SSIM &  & 33.52/0.926 & 33.43/0.926 & 29.17/0.895 & 34.55/0.939 & \best{34.77}/\best{0.942} & \\

        \begin{subfigure}[b]{0.2\linewidth}
            \includegraphics[width=\textwidth]{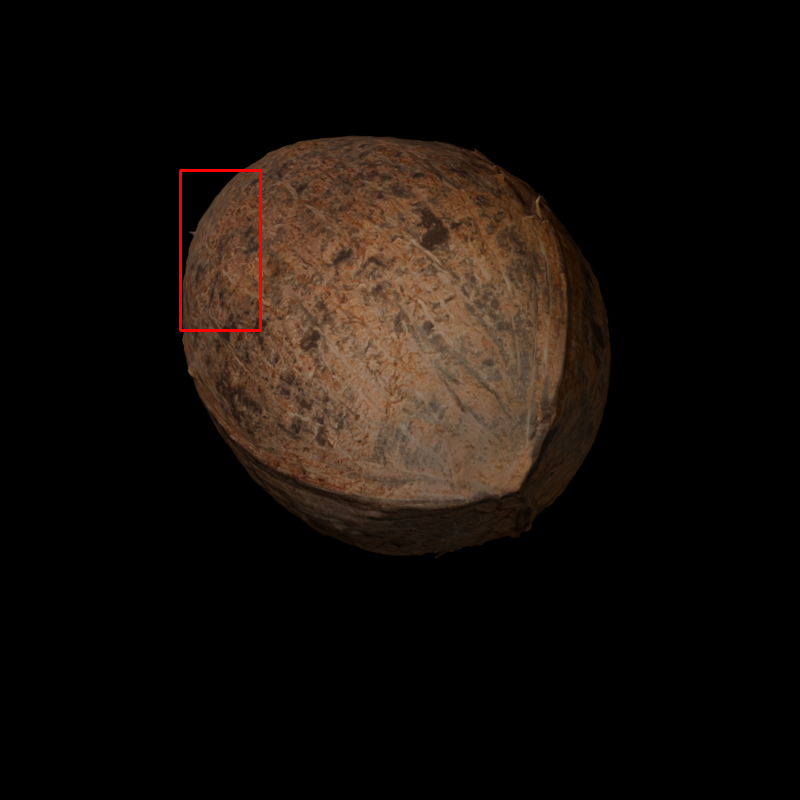}
            % \caption{Seed}
        \end{subfigure} &
        \begin{subfigure}[b]{0.1\linewidth}
            \includegraphics[width=\textwidth]{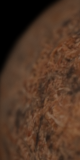}
            % \caption{}
        \end{subfigure} &  
        \begin{subfigure}[b]{0.1\linewidth}
            \includegraphics[width=\textwidth]{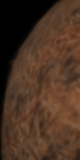}
            % \caption{}
        \end{subfigure} &
        \begin{subfigure}[b]{0.1\linewidth}
            \includegraphics[width=\textwidth]{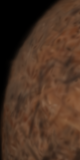}
            % \caption{}
        \end{subfigure} &
        \begin{subfigure}[b]{0.1\linewidth}
            \includegraphics[width=\textwidth]{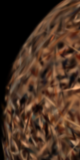}
            % \caption{}
        \end{subfigure} &
        \begin{subfigure}[b]{0.1\linewidth}
            \includegraphics[width=\textwidth]{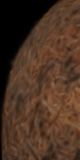}
            % \caption{}
        \end{subfigure} &   
        \begin{subfigure}[b]{0.1\linewidth}
            \includegraphics[width=\textwidth]{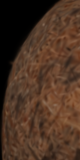}
            % \caption{}
        \end{subfigure} &  
        \begin{subfigure}[b]{0.1\linewidth}
            \includegraphics[width=\textwidth]{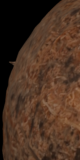}
            % \caption{}
        \end{subfigure} \\ 

        PSNR/SSIM &  & 38.87/0.957 & 38.74/0.957 & 29.49/0.884 & 39.82/0.970 & \best{40.26}/\best{0.974} & \\

        \begin{subfigure}[b]{0.2\linewidth}
            \includegraphics[width=\textwidth]{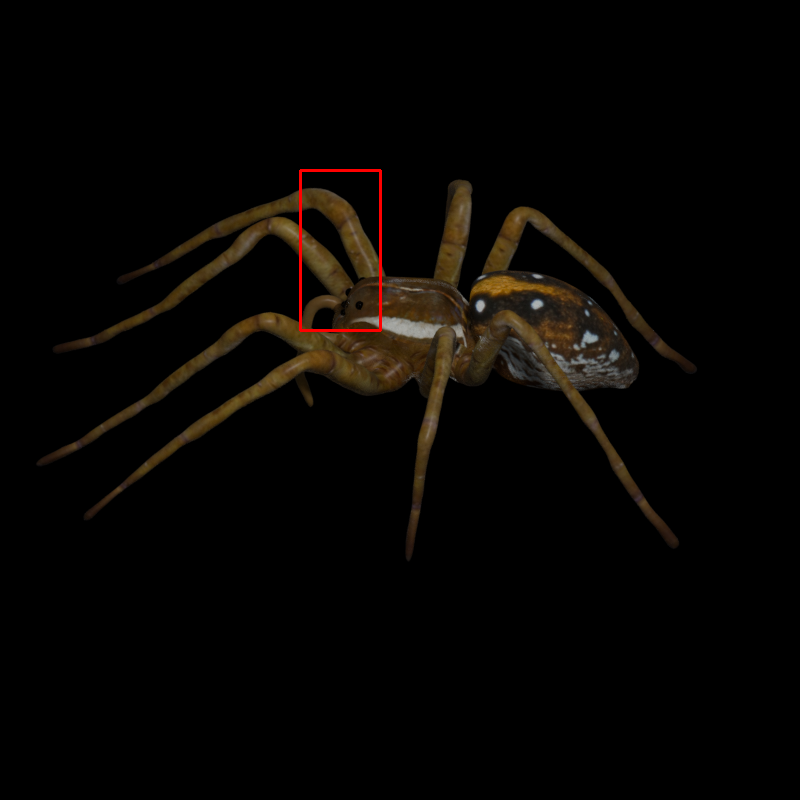}
            % \caption{Grain}
        \end{subfigure} &
        \begin{subfigure}[b]{0.1\linewidth}
            \includegraphics[width=\textwidth]{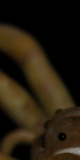}
            % \caption{}
        \end{subfigure} &  
        \begin{subfigure}[b]{0.1\linewidth}
            \includegraphics[width=\textwidth]{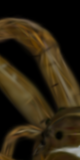}
            % \caption{}
        \end{subfigure} &
        \begin{subfigure}[b]{0.1\linewidth}
            \includegraphics[width=\textwidth]{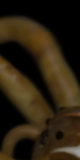}
            % \caption{}
        \end{subfigure} &
        \begin{subfigure}[b]{0.1\linewidth}
            \includegraphics[width=\textwidth]{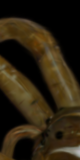}
            % \caption{}
        \end{subfigure} &
        \begin{subfigure}[b]{0.1\linewidth}
            \includegraphics[width=\textwidth]{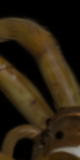}
            % \caption{}
        \end{subfigure} &   
        \begin{subfigure}[b]{0.1\linewidth}
            \includegraphics[width=\textwidth]{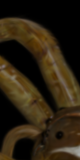}
            % \caption{}
        \end{subfigure} &  
        \begin{subfigure}[b]{0.1\linewidth}
            \includegraphics[width=\textwidth]{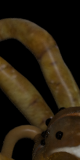}
            % \caption{}
        \end{subfigure} \\

        PSNR/SSIM &  & 37.76/0.970 & 37.35/0.965 & \best{38.00}/\best{0.973} & 37.63/0.968 & 37.87/0.972 & \\

        % \hline
    \end{tabular}
    \caption{\textbf{Visual comparisons of ablation studies on synthetic dataset}. Each row shows the results of removing different components from our method: depth input (w/o depth), clarity mask (w/o mask), multi-stage training (w/o stages), and BlurNet architecture (w/o BlurNet). We color code the \best{\textbf{best}} results.}
    \label{fig:ablation_comparison}
    \vspace{-1.5em}
\end{figure*}

In an optical imaging system, optical lenses can be considered as a transfer function from 3D space to the imaging plane. The transfer function is essentially a low-pass filter with a narrower bandwidth in the blurred region (defocused region) than in the clear region (focused region)~\cite{LI2013147}. Therefore, the focused region has more high-frequency information than the defocused region. Based on that, the whole process can be divided into the following parts:

First, a simple mean filter \(\mathbf{F}_m\) is employed to blur the source image \(\mathbf{I}\), then the mean-filtered image \(\text{MF}(\mathbf{I})\) is generated. That is,
\begin{equation}
  \text{MF}(\mathbf{I}) = \mathbf{F}_m \circ \mathbf{I},
  \label{eqsup5}
\end{equation}
where \(\mathbf{F}_m\) is the mean filter defined by
\begin{equation}
  (\mathbf{F}_m \circ \mathbf{I})[\mathbf{p}] = \sum_{i=-M}^{M}\sum_{j=-M}^{M}\frac{1}{(2M+1)^2}\mathbf{I}[\mathbf{p}+(i,j)],
  \label{eqsup6}
\end{equation}
where \(\mathbf{p}\) is a pixel in the image \(\mathbf{I}\), and \(M=3\) in our case.

Then, compared to the focus region of \(\mathbf{I}\), the corresponding region of \(\text{MF}(\mathbf{I})\) is blurred. The absolute value map of the difference between them is calculated to extract part of high-frequency information, which is regarded as the coarse in-focus map. It can be written as,
\begin{equation}
  \mathbf{M}_c = |\mathbf{I} - \text{MF}(\mathbf{I})|.
  \label{eqsup7}
\end{equation}

Finally, the guided filter~\cite{6319316} is used to enhance the high-frequency information of the coarse in-focus map \(\mathbf{M}_c\) with source image \(\mathbf{I}\) serving as the guidance image. Therefore, we obtain the fine in-focus map \(\mathbf{M}_f\), which has more high-frequency information than \(\mathbf{M}_c\), \ie,
\begin{equation}
  % \mathbf{M}_f = \text{GF}(\mathbf{I}, \mathbf{M}_c).
  \mathbf{M}_f[\mathbf{p}] = \sum_{\mathbf{q}\in\mathbf{M}_c}W_{\mathbf{p}\mathbf{q}}(\mathbf{I})\mathbf{M}_c[\mathbf{q}],
  \label{eqsup8}
\end{equation}
where \(W_{\mathbf{p}\mathbf{q}}(\mathbf{I})\) is defined as
\begin{equation}
  W_{\mathbf{p}\mathbf{q}}(\mathbf{I}) = \frac{1}{|\omega|^2}\sum_{\omega_k \in \mathcal{K}_{\mathbf{p}\mathbf{q}}}\left(1+\frac{(\mathbf{I}[\mathbf{p}]-\mu_k)(\mathbf{I}[\mathbf{q}]-\mu_k)}{\sigma_k^2+\epsilon}\right),
  \label{eqsup9}
\end{equation}
where \(\omega\) is a window with size \(R\times R\), \(\mu_k\) and \(\sigma_k^2\) are the mean and variance of the window \(\omega_k\). \(\mathcal{K}_{\mathbf{p}\mathbf{q}}\) is set of all windows containing pixels \(\mathbf{p}\) and \(\mathbf{q}\) at the same time. \(\epsilon\) is a regularization parameter. We set \(R=5\) and \(\epsilon=0.3\) in our case.

Through this, we get a fine in-focus map \(\mathbf{M}_f\), which can serve as the clarity mask \(\mathbf{M}\) in our method.

\begin{figure*}[htb!]
    \setlength{\abovecaptionskip}{3pt}
    \setlength{\tabcolsep}{1pt}
    \centering
    \small
    \begin{tabular}[b]{ccccc}
        
        Iteration 3000 & Iteration 15000 & Iteration 25000 & Iteration 30000 & Ground Truth \\
        
        \begin{subfigure}[b]{0.2\linewidth}
            \includegraphics[width=\textwidth]{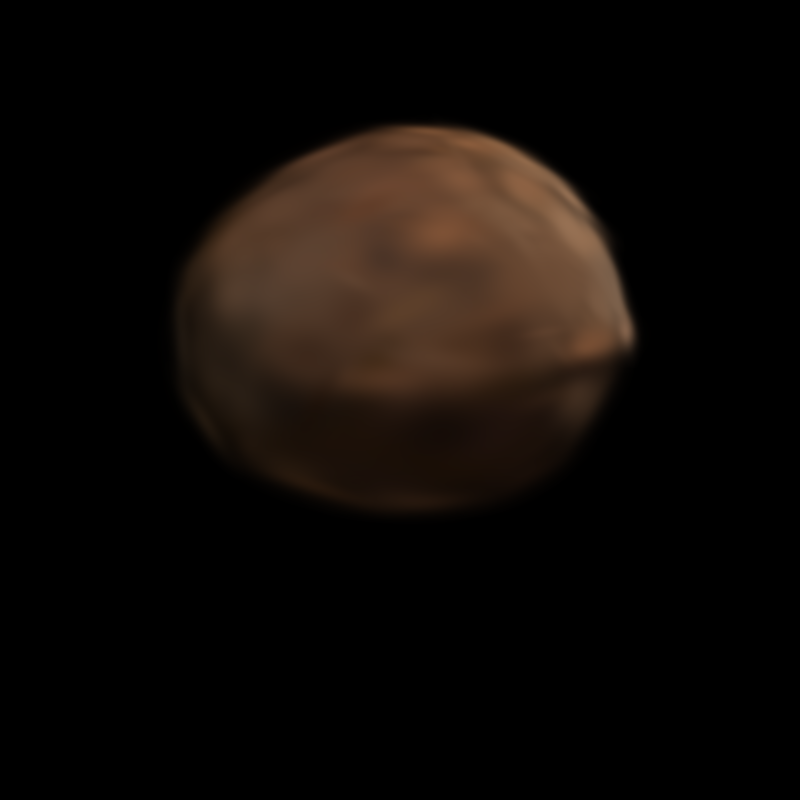}
            % \caption{3K}
        \end{subfigure} &
        \begin{subfigure}[b]{0.2\linewidth}
            \includegraphics[width=\textwidth]{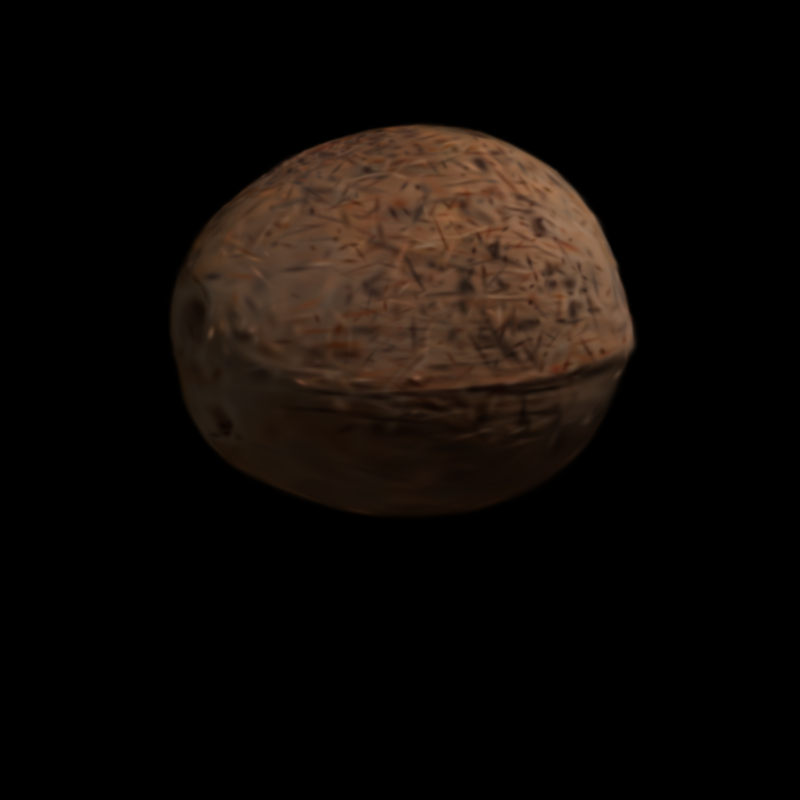}
            % \caption{15K}
        \end{subfigure} &  
        \begin{subfigure}[b]{0.2\linewidth}
            \includegraphics[width=\textwidth]{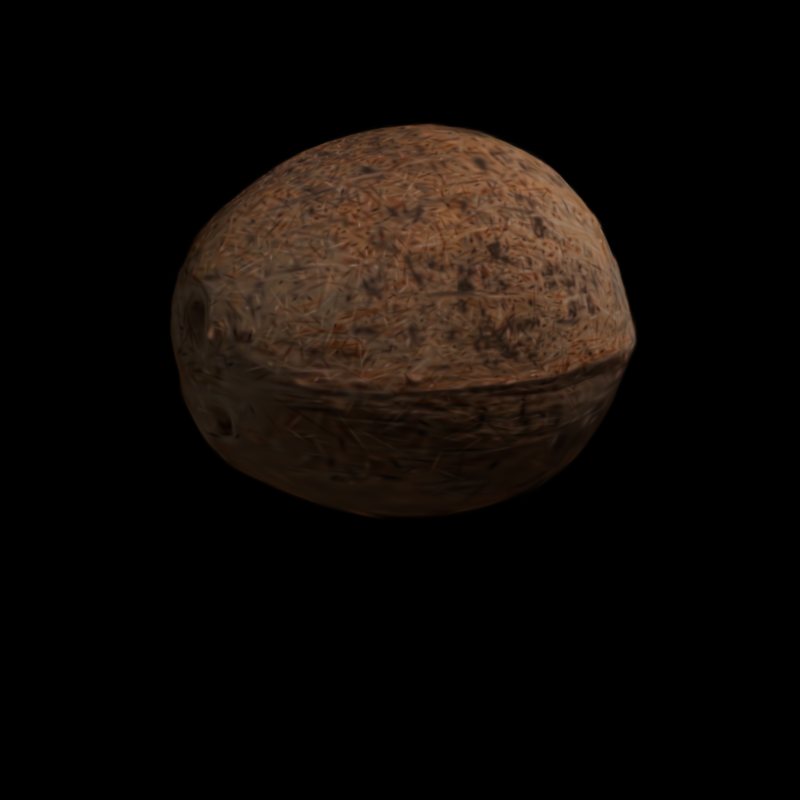}
            % \caption{25K}
        \end{subfigure} &
        \begin{subfigure}[b]{0.2\linewidth}
            \includegraphics[width=\textwidth]{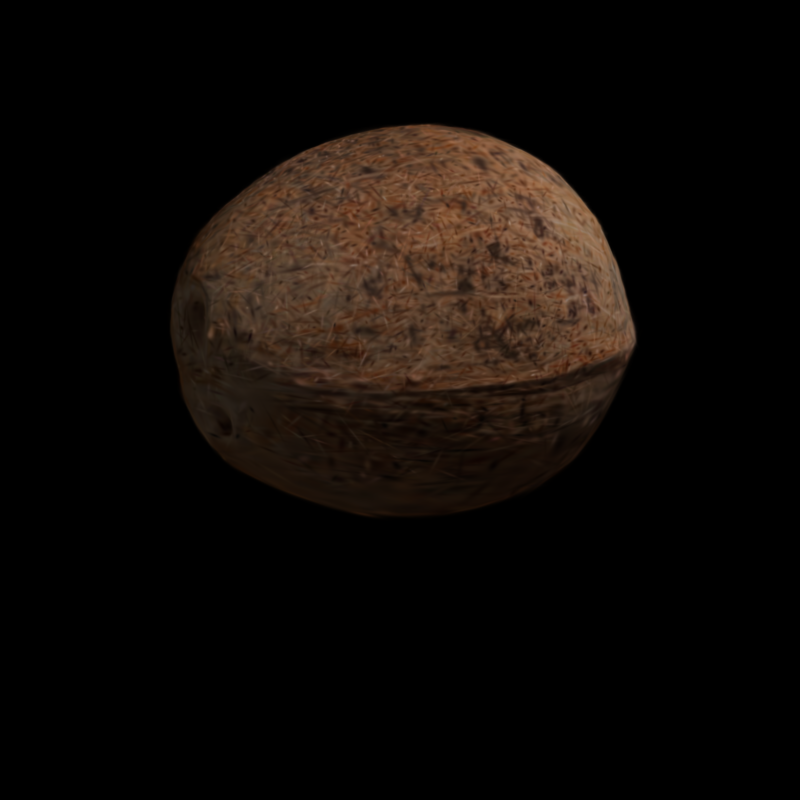}
            % \caption{30K}
        \end{subfigure} &
        \begin{subfigure}[b]{0.2\linewidth}
            \includegraphics[width=\textwidth]{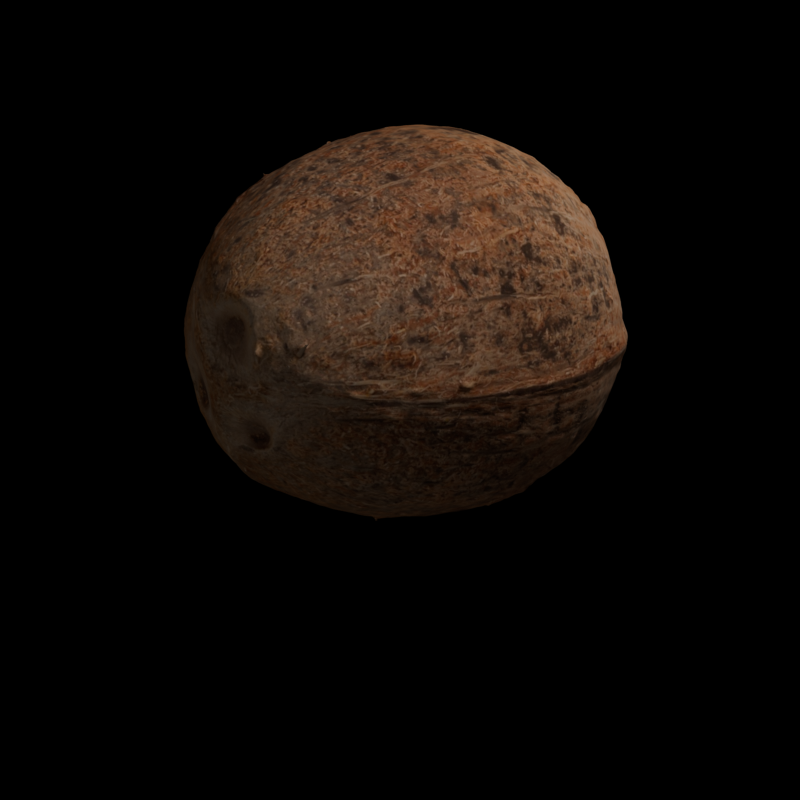}
            % \caption{GT}
        \end{subfigure} \\
        
        \multicolumn{5}{c}{Ours} \\
        
        \begin{subfigure}[b]{0.2\linewidth}
            \includegraphics[width=\textwidth]{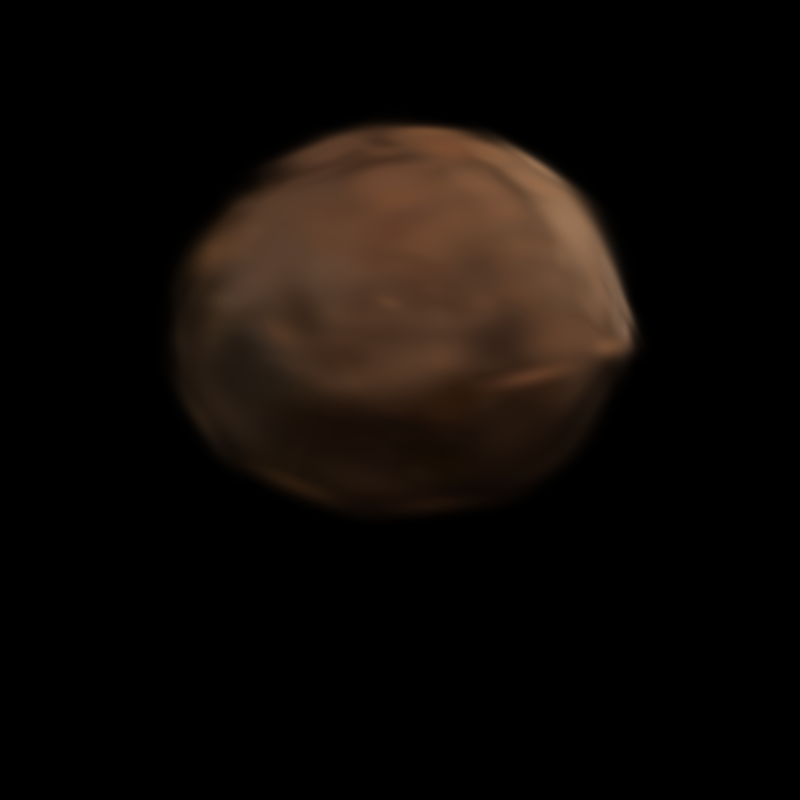}
            % \caption{3K}
        \end{subfigure} &
        \begin{subfigure}[b]{0.2\linewidth}
            \includegraphics[width=\textwidth]{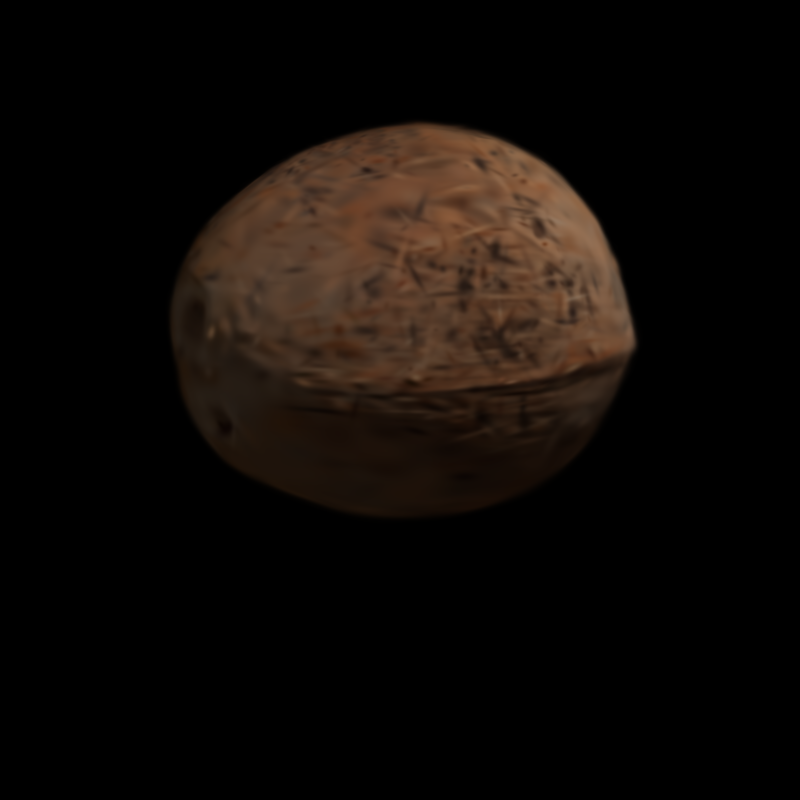}
            % \caption{15K}
        \end{subfigure} &  
        \begin{subfigure}[b]{0.2\linewidth}
            \includegraphics[width=\textwidth]{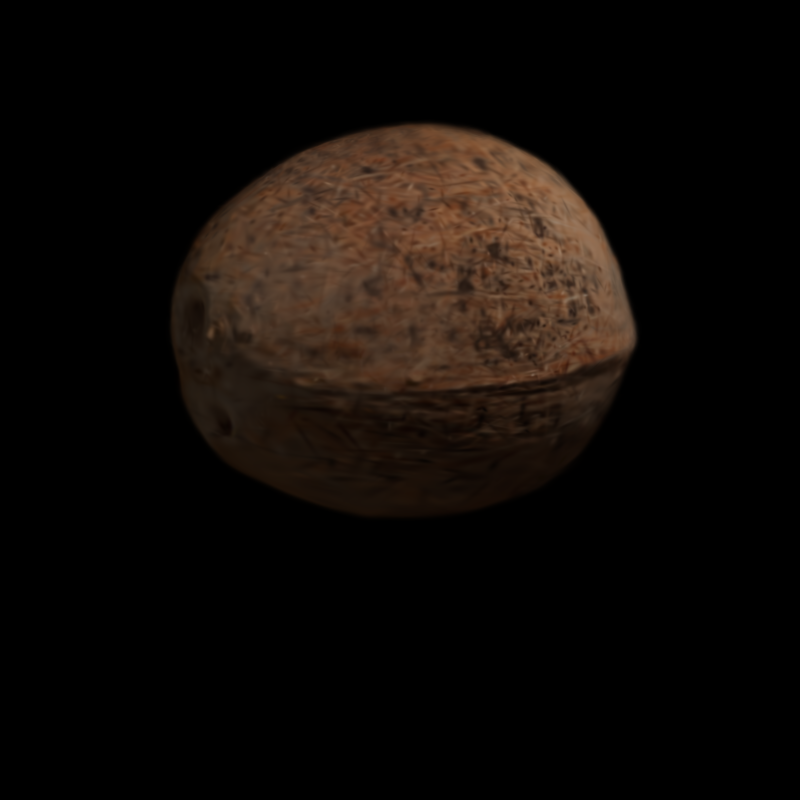}
            % \caption{25K}
        \end{subfigure} &
        \begin{subfigure}[b]{0.2\linewidth}
            \includegraphics[width=\textwidth]{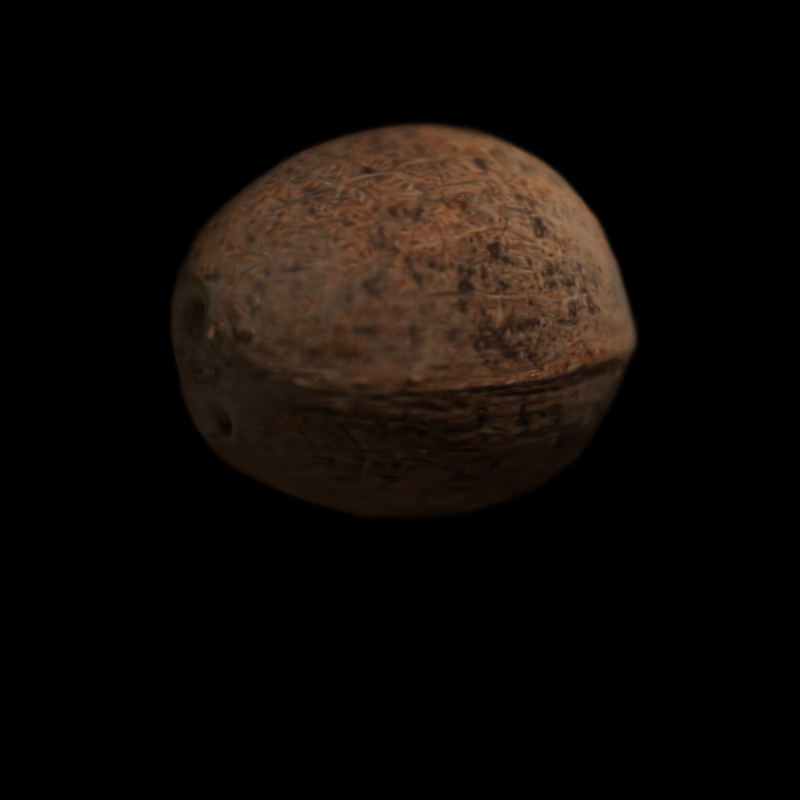}
            % \caption{30K}
        \end{subfigure} &
        \begin{subfigure}[b]{0.2\linewidth}
            \includegraphics[width=\textwidth]{imgs/training_comparison/gt.png}
            % \caption{GT}
        \end{subfigure} \\
        
        \multicolumn{5}{c}{3DGS Baseline} \\
        
    \end{tabular}
    \caption{\textbf{Training progression comparison between our method and 3DGS baseline}. The visualization demonstrates how our method progressively recovers sharp details from blurry inputs across different training iterations, while the 3DGS baseline struggles to achieve clear reconstruction from the same blurry inputs.}
    \label{fig:training_progression}
    \vspace{-1.5em}
\end{figure*}

\section{More Implementation Details}
\label{sec:moredetails}

\subsection{Synthetic dataset.}
we use the built-in aperture functionality in Blender~\cite{misc_blender} to simulate defocus blur. We measure that the focal plane depth \(d_0\) to the object depth change \(\epsilon_{\mathbf{p}}\) in real macrophotography scenes is about 100:1, so we scale the object size to [-1,1] and set the distance between the camera and the object to 100. Experience shows that when the aperture value is set to 0.12, the defocus blur effect of the rendered image is closest to the real microscopic image. We add a small perturbation that follows a normal distribution to the distance between the camera and the object to simulate subtle changes in the focal plane and verify the robustness of our method to depth.

\vspace{-3mm}
\subsection{Real-world dataset.}
Since real tiny objects are too small and the field of view of the macro camera is also small, it is easy for the object to leave the field of view of the camera when the camera is moved. Therefore, we choose to fix the camera and attach the object to a rotatable device. Fig.~\ref{fig:rebuttal_scene} shows the capture device of our real dataset, which ensures quality and speed of capturing. The system captures an image every 3 degrees of rotation. After rotating 360 degrees, the object is attached to the rotatable device in different poses, and 2 or 3 sets of images are taken for each object in this way. After the capturing is completed, we use Agisoft~\cite{AgiSoftPhotoScan} to calculate the camera posture and convert it into a form that can be read by COLMAP~\cite{misc_colmap1, misc_colmap2} to check whether the result is correct.

\begin{table}[htbp]
    \centering
    \resizebox{\linewidth}{!}{
    % \resizebox{0.42\textwidth}{!}{

    \begin{tabular}{l |cccccc}

     Methods  & \multicolumn{3}{c}{DbGS \cite{lee2024deblurring3dgs}}  & \multicolumn{3}{c}{DbGS-adjusted} \\

     Metrics & PSNR & SSIM & LPIPS & PSNR & SSIM & LPIPS  \\

     \midrule[1pt]

    Seed & 22.75 & 0.820 & 0.154 & \best{38.56} & \best{0.953} & \best{0.092}  \\
    Micro-Chair & 14.52 & 0.861 & 0.151 & \best{27.29} & \best{0.926} & \best{0.075}  \\
    
    \end{tabular}
}    
    % \caption{Quantitative comparisons on the micro scenarios dataset. We color code the \colorbox[HTML]{FD6864}{\textbf{best}} and \colorbox[HTML]{FFCE93}{\textbf{second best}}.}
    \caption{\textbf{Quantitative comparisons on the adjustments to Deblurring-3DGS.} We color code the \best{\textbf{best}}.}
    \label{tab:dbgs}

% \vspace{-2em}
\vspace{-0.2cm}
\end{table}

\vspace{-3mm}
\subsection{Comparative experiments setting.}
In the comparative experiments, in order to make other methods applicable to macro scenes and keep the parameters consistent, we adjusted some methods. For Deblurring-3DGS~\cite{lee2024deblurring3dgs}, we deleted the algorithm of adding points in the background and adjusted the adaptive density control to make it consistent with 3DGS~\cite{kerbl20233dgs}. As shown in Tab.~\ref{tab:dbgs}, these changes improve the performance of Deblurring-3DGS in macro scenes. We believe that this improvement reflects the difference between natural scenes and macro scenes. In macrophotography, due to the sensitivity to depth, defocus blur occurs near the focal plane, while there are usually no objects far from the focal plane, so there is no need for additional modeling of the background. In addition, we set the number of iterations of Deblurring-3DGS to 30,000 and the number of iterations of BAGS~\cite{peng2024bags} to 36,000 (the first 6,000 of which are pre-training) to keep the number of iterations consistent.

\section{Additional Visualization Results}
\label{sec:additional_vis}

This section provides additional visualization results to support our main experimental conclusions, which contain two parts: ablation study visualizations and training process visualizations.

\subsection{Ablation Study Visualizations}
\label{subsec:ablation_vis}

Fig.~\ref{fig:ablation_comparison} presents detailed visual comparisons of our ablation studies on synthetic datasets. The visualization demonstrates the individual contribution of each component in our method.

The visual results clearly show that our full method achieves the sharpest reconstruction with the richest details, validating the effectiveness of each proposed component.

\subsection{Training Process Visualizations}
\label{subsec:training_vis}

Fig.~\ref{fig:training_progression} illustrates the evolution of our self-supervised optimization process compared with 3DGS baseline. The visualization captures the progressive improvement of our method across different training iterations, demonstrating how our joint deblurring and reconstruction approach gradually recovers sharp details from blurry inputs while the baseline method struggles with the same challenging inputs.
